# Supplementary material for: Enhancement of Electric Drive in Silicon Quantum Dots with Electric Quadrupole Spin Resonance
Source: arXiv:2502.01040 ancillary file (2025-10-09)
Supplement: Supplementary file 1 [file EQSR_Supplementary.pdf]

# Supplementary Material: Enhancement of Electric Drive in Silicon Quantum Dots with Electric Quadrupole Spin Resonance

Philip Y. Mai,<sup>1,\*</sup> Pedro H. Pereira,<sup>2,\*</sup> Lucas Andrade Alonso,<sup>2,\*</sup> Ross C. C. Leon,<sup>1,†</sup> Chih Hwan Yang,<sup>1,3</sup> Jason C. C. Hwang,<sup>1</sup> Daniel Dunmore,<sup>1</sup> Julien Camirand Lemyre,<sup>4</sup> Tuomo Tantt,<sup>1,3</sup> Wister Huang,<sup>1,‡</sup> Kok Wai Chan,<sup>1,3</sup> Kuan Yen Tan,<sup>1,§</sup> Jesús D. Cifuentes,<sup>1</sup> Fay E. Hudson,<sup>1,3</sup> Kohei M. Itoh,<sup>5</sup> Arne Laucht,<sup>1,3</sup> Michel Pioro-Ladrière,<sup>4,6</sup> Christopher C. Escott,<sup>1,3</sup> MengKe Feng,<sup>1,¶</sup> Reinaldo de Melo e Souza,<sup>2</sup> Andrew Dzurak,<sup>1,3</sup> and Andre Saraiva<sup>1,3,\*\*</sup>

<sup>1</sup>*School of Electrical Engineering and Telecommunications,  
The University of New South Wales, Sydney, NSW 2052, Australia*

<sup>2</sup>*Instituto de Física, Universidade Federal Fluminense, 24210-346, RJ, Brazil*

<sup>3</sup>*Diraq, Sydney, NSW 2052, Australia*

<sup>4</sup>*Institut Quantique et Département de Physique,  
Université de Sherbrooke, Sherbrooke, Québec, J1K 2R1, Canada*

<sup>5</sup>*School of Fundamental Science and Technology, Keio University,  
3-14-1 Hiyoshi, Kohokuku, Yokohama, 223-8522, Japan*

<sup>6</sup>*Quantum Information Science Program, Canadian Institute for Advanced Research, Toronto, ON, M5G 1Z8, Canada*

## DETAILS OF THE EFFECTIVE SINGLE-PARTICLE HAMILTONIAN

In this section, we elaborate on the effective system Hamiltonian defined in the main text. There are a few characteristics of the system that informed us of how to construct the Hamiltonian. Firstly, an integrated micromagnet was introduced into the device to facilitate electric driving [1] and as a result, for 5 and 13 electron occupancies, faster Rabi oscillations via electric dipole spin resonance and an improvement in the single-qubit gate fidelity could be achieved, compared to the single electron regime [2]. However, electric dipole effects alone cannot explain those improvements, and a more careful treatment of the qubit dynamics must be made.

Secondly, as briefly mentioned in the main text, the multi-electron dot in Ref. [2] exhibits a regular shell structure which can be predicted from single-particle theory – namely closed-shell configurations at 4, 12, 24, ... electrons due to the 2D confinement and the spin and valley degeneracy [3]. This suggests that the Coulomb interaction can be regarded as a perturbation upon the single particle Hamiltonian. Otherwise, the spectrum would appear vastly different due to highly-correlated states such as Wigner molecules [4, 5]. As such, we model the dot by an effective single-particle, 2D Hamiltonian that describes the low-energy physics.

The hamiltonian described in the main text is a simplification of the one used to perform our simulations. Here, we will comment on the full  $H_{\text{DC}}$  Hamiltonian, including terms omitted in the main text. We have

$$H_{\text{DC}} = H_{\text{xy}} + H_{\text{Zee}} + H_{\text{SO}} + H_{\text{mm}} + H_{\text{an}} + H_{\text{para}} + H_{\text{dia}} + H_{\eta}. \quad (\text{S1})$$

The last five terms were not shown in the main text and will be explained in this section.

Considering a lateral confinement provided by an anisotropic parabolic potential, the orbital motion in effective mass theory is described by [6–8]

$$H_{\text{orb}} = \sum_i \frac{\pi_i^2}{2m_i^*} + \frac{1}{2}m_t(\omega_x^2 x^2 + \omega_y^2 y^2) + U_0\Theta(z) - eE_z z, \quad (\text{S2})$$

where  $i \in \{x, y, z\}$ ,  $\pi_i$  is the canonical momentum in the  $i$  direction,  $U_0\Theta(z)$  models the shift in the conduction band minimum at the Si/SiO<sub>2</sub> interface, and  $eE_z z$  accounts for the vertical confinement of electrons near this interface (2DEG). As the energy necessary to excite an electron in the  $z$  direction is much larger than the ones necessary to excite it in the  $x$  and  $y$  directions, we will consider that the wave function is frozen in the  $z$  direction. This means that every  $z$  operator can be substituted to its expected value in the stationary state  $\langle z \rangle = -2.01\text{nm}$  and we can consider only the orbital Hamiltonian in the  $x$  and  $y$  directions, as in Eq. 2 in the main text. The vertical confinement splits the degenerate  $\Delta$  valleys  $|\pm k_0\rangle$  due to the sharp Si/SiO<sub>2</sub> interface but is neglected in our model because they are not important for describing most of the physics.

The presence of a magnetic field is taken into account by the replacement  $\pi_i \rightarrow p_i + eA_i$ , where  $A_i$  stands for the

$i$ -th component of the vector potential [9]. The gauge choice that better suits our purpose is

$$\mathbf{A} = \begin{pmatrix} zB_y - \frac{1}{2}B_z y \\ -zB_x + \frac{1}{2}B_z x \\ 0 \end{pmatrix} \quad (\text{S3})$$

as proposed by Stano et. al [10], which leads to

$$H_{\text{orb}} = H_{xy} + H_{\text{para}} + H_{\text{dia}} \quad (\text{S4})$$

after some calculations, where

$$H_{\text{para}} = \frac{eB_z}{2m_l}(xp_y - yp_x) \quad (\text{S5})$$

$$H_{\text{dia}} = \frac{e^2 B_z^2}{8m_l}(x^2 + y^2) \quad (\text{S6})$$

are the called paramagnetic and diamagnetic hamiltonians and  $H_{xy}$  is stated in the main text. The total magnetic field  $\mathbf{B}$  is composed by the external field  $\mathbf{B}_0 = -B_0\hat{y}$  mentioned in the main text and the field gradient produced by a micromagnet, given by  $\mathbf{B}_{\text{mm}} = b(z - y)\hat{y} + b(z + y)\hat{z}$ , with  $b$  being the slope of the gradient. Therefore,  $B_z = b(z + y)$ . The micromagnetic main effect, however, shows when calculating the Zeeman effect it produces, yielding the hamiltonian

$$H_{\text{mm}} = \frac{g\mu_B}{2}\mathbf{B}_{\text{mm}} \cdot \boldsymbol{\sigma} \quad (\text{S7})$$

$$= \frac{g\mu_B b}{2}(z - y)\sigma_y + (z + y)\sigma_z, \quad (\text{S8})$$

which is a extrinsic spin-orbit coupling, offering us products of orbital and spin degrees of freedom in a similar way to  $H_{\text{SO}}$ , allowing the necessary state hybridization mentioned in the main text.

An anarmonicicity is present in the lateral confinement potential, which we can model with the hamiltonian

$$H_{\text{an}} = \lambda_{xy}xy. \quad (\text{S9})$$

In addition, we will also consider the effect of linear Stark shift arising from spin-orbit effects on the Zeeman energy. This effect can be observed in Fig. 3 (in both the 5 and 13 electron case) where the qubit frequency has an approximately linear dependence on the ellipticity,  $\delta$ . To account for this effect, we include an additional term in our fitting, corresponding to a shift in the Zeeman energy as a function of  $\delta$ ,

$$H_{\text{Zee}} = H_{\text{Zee}}[1 + \eta(\delta - 1)] , \quad (\text{S10})$$

where the Zeeman Hamiltonian is effectively shifted by an amount given by  $\eta$  which is the linear Stark shift and the deviation away from  $\delta = 1$ , which is the point of minimum ellipticity.  $\eta$  is a fitting parameter in the simulations.

## FITTING PROTOCOL AND FITTED VALUES

To obtain the plots shown in Fig. 4 in the main text, we perform a fitting similar to that which was described in Ref. [11]. In the fitting algorithm, we are fitting all nine parameters as shown in Tab. S1 simultaneously, which all enter the full Hamiltonian as described in the main text. The algorithm then extracts the two metrics of concern, which are the qubit frequencies  $f_{\text{ESR}}$ , given by  $hf_{\text{ESR}} = \mathcal{E}_1 - \mathcal{E}_0 - hf_{\text{ESR},0}$ , where  $f_{\text{ESR},0}$  is a fitting parameter, and the Rabi frequency  $\Omega$  given by Eq. (9).

We perform a least-squares fit to the experimental data, simultaneously fitting both the qubit and Rabi frequencies as a function of  $\delta$ , assuming the relation

$$\delta = \delta_1 V_{\text{G2}} + \delta_0 \quad (\text{S11})$$

| Parameter                             | Fitted Value (5e)            | Fitted Value (13e)             |
|---------------------------------------|------------------------------|--------------------------------|
| $eQ_{xy}$ (meV/nm <sup>2</sup> )      | $(2 \pm 8) \times 10^{-6}$   | $(4 \pm 3) \times 10^{-6}$     |
| $\alpha$ (meV nm)                     | $-2 \pm 2$                   | $-1.6 \pm 0.8$                 |
| $\beta$ (meV nm)                      | $2 \pm 2$                    | $1.5 \pm 0.8$                  |
| $\hbar\omega_y$ (meV)                 | $4 \pm 4$                    | $11 \pm 3$                     |
| $f_{\text{ESR},0}$ (MHz)              | $(1 \pm 9) \times 10^1$      | $(2 \pm 2) \times 10^1$        |
| $\lambda_{xy}$ (meV/nm <sup>2</sup> ) | $(2 \pm 2) \times 10^{-3}$   | $(4 \pm 1) \times 10^{-3}$     |
| $\delta_0$                            | $1.050 \pm 0.006$            | $1.0063 \pm 0.0001$            |
| $\eta$                                | $(-1 \pm 3) \times 10^{-3}$  | $(1.0 \pm 0.1) \times 10^{-3}$ |
| $b$ (mVs/nm <sup>3</sup> )            | $(4 \pm 18) \times 10^{-19}$ | $(4 \pm 3) \times 10^{-19}$    |

Table S1. Fitted values with 95% confidence intervals.

where  $V_{G2}$  is the voltage in the electrostatic gate responsible for the lateral qubit confinement,  $\delta_0$  is the voltage at which the degeneracy occurs and is a fitting parameter, and  $\delta_1$  describes the effect of  $V_{G2}$  on ellipticity  $\delta$ , as shown in Fig. 2(b). We calculated  $\delta_1$  from Fig. 2(b) for the different electron regimes, with  $-0.54 \text{ V}^{-1}$  for 5 electrons and  $-0.38 \text{ V}^{-1}$  for 13 electrons.

The cost function that is being minimized is a function of the squared differences between the calculated metrics and the experimentally obtained values.

We note that differences in both the number of data points as well as the magnitude of the metrics themselves influence the weightage of the qubit frequencies and the Rabi frequencies during the fitting. We use trial and error to either magnify or diminish their weights in order that both metrics are fitted on almost equal footing.

We also note that in the main text, we presented results in Fig. 4, showing that we were able to obtain fits of both the qubit frequency and the Rabi frequency using the above-described fitting protocol while taking into account EQSR.

Here, we will elaborate on the technical aspects of the fitting that made it difficult to obtain a quantitative fit. The first is that despite having experimental data, it was not taken with this theoretical analysis in mind, which means that there remains much unknown about the system. This leaves several free-fitting parameters that will have to be fitted simultaneously (in this case, nine). In addition, while we can use physical intuition to guess the order of magnitudes for these parameters, it often becomes difficult to ascertain their actual values. This becomes especially tricky in cases where two different parameters can have opposing effects and the fitting algorithm will find it difficult to find a global minimum. The sheer number of free parameters coupled with insufficient experimental data points add to the difficulty of obtaining ideal fits. In future similar studies, this difficulty can be overcome by both increasing the number of data points taken, as well as making use of more experiments to ascertain some of the fitting parameters independently, which goes a long way towards simplifying the fit.

## DEFINING COORDINATE SYSTEM

Here, we describe and explain the coordinate transformation used in the main text. Generally, caution is advised when analyzing the Hamiltonians described, since there are three different coordinate systems: (i) the orbital/real space coordinates, defined by the electrostatic confinement, as in Eq. 2, (ii) the spin coordinates, defined by the external magnetic field  $B_0$ ; (iii) the crystallographic coordinates, defined by the orientation of the crystal, as in Eq. 3. We will refer to them as  $\{x, y, z\}$ ,  $\{x', y', z'\}$  and  $\{x^C, y^C, z^C\}$ , respectively. The direction of the spin is chosen such that  $z' \parallel B_0 \parallel -y$ ; the crystallographic axis [110] is chosen to be oriented as well in the  $-y$  direction. Hence, the coordinate systems are related through the equations:

$$x^C = -\frac{(x+y)}{\sqrt{2}}, y^C = \frac{x-y}{\sqrt{2}}, z^C = z, \quad (\text{S12})$$

$$x' = x, y' = z, z' = -y, \quad (\text{S13})$$

$$x^C = \frac{z' - x'}{\sqrt{2}}, y^C = \frac{z' + x'}{\sqrt{2}}, z^C = y'. \quad (\text{S14})$$

where we define the crystallographic axis in real space coordinates (Eq. S12), and also the spin coordinates in real space coordinates (Eq. S13), therefore allowing us to define in Eq. S14 the crystallographic coordinates in spin coordinates.

The spin-orbit Hamiltonian is usually stated in literature as

$$H_{\text{SO}} = \alpha \underbrace{(\sigma_x^C k_y^C - \sigma_y^C k_x^C)}_{h_{\text{R}}} + \beta \underbrace{(\sigma_x^C k_x^C - \sigma_y^C k_y^C)}_{h_{\text{D}}}. \quad (\text{S15})$$

The Rashba term in this equation can then be written as

$$h_{\text{R}} = \sigma_x^C k_y^C - \sigma_y^C k_x^C \quad (\text{S16})$$

$$= \frac{1}{2}(\sigma'_z - \sigma'_x)(k_x - k_y) + \frac{1}{2}(\sigma'_z + \sigma'_x)(k_x + k_y) \quad (\text{S17})$$

$$= k_x \sigma'_z + k_y \sigma'_x. \quad (\text{S18})$$

Similarly, the Dresselhaus term becomes

$$h_{\text{D}} = -k_x \sigma'_z + k_y \sigma'_x. \quad (\text{S19})$$

Therefore obtaining the form used in Eq. 3 in the main text.

---

\* These authors contributed equally

† Current Address: Quantum Motion, 9 Sterling Way, London N7 9HJ, United Kingdom

‡ Current Address: Laboratory for Solid State Physics, ETH Zurich, CH-8093 Zurich, Switzerland

§ Current Address: IQM Quantum Computers, Espoo 02150, Finland

¶ mengke.feng@unsw.edu.au

\*\* a.saraiva@unsw.edu.au

- [1] M. Pioro-Ladrière, Y. Tokura, T. Obata, T. Kubo, and S. Tarucha, *Applied Physics Letters* **90**, 024105 (2007).
- [2] R. Leon, C. H. Yang, J. Hwang, J. C. Lemyre, T. Tanttu, W. Huang, K. W. Chan, K. Tan, F. Hudson, K. Itoh, *et al.*, *Nature communications* **11**, 797 (2020).
- [3] C. H. Yang, A. Rossi, R. Ruskov, N. S. Lai, F. A. Mohiyaddin, S. Lee, C. Tahan, G. Klimeck, A. Morello, and A. S. Dzurak, *Nature Communications* **4**, 1 (2013).
- [4] J. Corrigan, J. Dodson, H. E. Ercan, J. Abadillo-Uriel, B. Thorgrimsson, T. Knapp, N. Holman, T. McJunkin, S. F. Neyens, E. MacQuarrie, R. H. Foote, L. Edge, M. Friesen, S. Coppersmith, and M. Eriksson, *Physical Review Letters* **127**, 10.1103/physrevlett.127.127701 (2021).
- [5] H. E. Ercan, S. N. Coppersmith, and M. Friesen, *Physical Review B* **104**, 10.1103/physrevb.104.235302 (2021).
- [6] A. L. Saraiva, M. J. Calderón, R. B. Capaz, X. Hu, S. D. Sarma, and B. Koiller, *Physical Review B* **84**, 155320 (2011).
- [7] R. Ruskov, M. Veldhorst, A. S. Dzurak, and C. Tahan, *Physical Review B* **98**, 10.1103/physrevb.98.245424 (2018).
- [8] M. Veldhorst, R. Ruskov, C. H. Yang, J. C. C. Hwang, F. E. Hudson, M. E. Flatté, C. Tahan, K. M. Itoh, A. Morello, and A. S. Dzurak, *Physical Review B* **92**, 201401 (2015).
- [9] L. E. Ballentine, *Quantum mechanics: a modern development* (World Scientific Publishing Company, 2014).
- [10] P. Stano, C.-H. Hsu, L. C. Camenzind, L. Yu, D. Zumbühl, and D. Loss, *Physical Review B* **99**, 085308 (2019).
- [11] W. Gilbert, T. Tanttu, W. H. Lim, M. Feng, J. Y. Huang, J. D. Cifuentes, S. Serrano, P. Y. Mai, R. C. Leon, C. C. Escott, *et al.*, *Nature Nanotechnology*, 1 (2023).
